# Supplementary material for: Radiative Decays of the Spin-$\nicefrac{3}{2}$ to Spin-$\nicefrac{1}{2}$ Doubly Heavy Baryons in QCD
Source: arXiv:2306.14552 source file (2023-06-26)
Supplement: Supplementary file 1 [file appendixA.tex]

\section{Photon Distribution Amplitudes}
\label{appndxa}
In this appendix, for completeness, we present the explicit expressions for the photon distribution amplitudes\cite{PhotonDA}.
\begin{align*}
        \bra{0}\overline{q}(x)\sigma_{\mu\nu}q(0)\ket{0}_F &= -ie_q\qbarq\left(\varepsilon_\mu q_\nu - \varepsilon_\nu q_\mu\right) \int_0^1 du e^{i\bar{u}qx}\left(\chi\varphi_\gamma(u)+\dfrac{x^2}{16}\mathbb{A}(u)\right) \nonumber \\
        &-\dfrac{i}{2(qx)}\left[x_\nu\left(\varepsilon_\mu - q_\mu\dfrac{\varepsilon x}{qx}\right) - x_\mu\left(\varepsilon_\nu - q_\nu\dfrac{\varepsilon x}{q x}\right)\right] \int_0^1 du e^{i\overline{u}qx}h_\gamma(u) \nonumber \\    
        \bra{0}\overline{q}(x)\gamma_\mu q(0)\ket{0}_F &= e_qf_{3\gamma}\left(\varepsilon_\mu-q_\mu\dfrac{\varepsilon x}{qx}\right) \int_0^1du e^{i\overline{u}qx}\psi^v(u)\\    
        \bra{0}\overline{q}(x)\gamma_\mu\gf q(0)\ket{0}_F &=-\dfrac{1}{4}e_qf_{3\gamma}\varepsilon_{\mu\nu\alpha\beta}\varepsilon^\nu q^\alpha x^\beta \int_0^1 du e^{i\overline{u}qx}\psi^a(u)\\   
        \bra{0}\overline{q}(x)g_sG_{\mu\nu}(vx)q(0)\ket{0}_F&=-ie_q\qbarq\left(\varepsilon_\mu q_\nu - \varepsilon_\nu q_\mu\right)\int \mathcal{D}\alpha_ie^{i(\alpha_{\Bar{q}}+v\alpha_g)qx}\mathcal{S}\left(\alpha_i\right)\\
        \bra{0}\overline{q}(x)F_{\mu\nu}(vx)q(0)\ket{0}_F&=-i\qbarq\left(\varepsilon_\mu q_\nu - \varepsilon_\nu q_\mu\right)\int \mathcal{D}\alpha_ie^{i(\alpha_{\Bar{q}}+v\alpha_g)qx}\mathcal{S}^\gamma\left(\alpha_i\right)\\ 
        \bra{0}\overline{q}(x)g_s\Tilde{G}_{\mu\nu}(vx)i\gf q(0)\ket{0}_F&=-ie_q\qbarq\left(\varepsilon_\mu q_\nu - \varepsilon_\nu q_\mu\right)\int \mathcal{D}\alpha_ie^{i(\alpha_{\Bar{q}}+v\alpha_g)qx}\Tilde{\mathcal{S}}\left(\alpha_i\right)\\   
        \bra{0}\overline{q}(x)g_s\Tilde{G}_{\mu\nu}(vx)\gamma_\alpha\gf q(0)\ket{0}_F&=e_qf_{3\gamma}\left(\varepsilon_\mu q_\nu - \varepsilon_\nu q_\mu\right)\int \mathcal{D}\alpha_ie^{i(\alpha_{\Bar{q}}+v\alpha_g)qx}\mathcal{A}\left(\alpha_i\right)\\   
        \bra{0}\overline{q}(x)g_sG_{\mu\nu}(vx)i\gamma_\alpha q(0)\ket{0}_F &=e_qf_{3\gamma}\left(\varepsilon_\mu q_\nu - \varepsilon_\nu q_\mu\right)\int \mathcal{D}\alpha_ie^{i(\alpha_{\Bar{q}}+v\alpha_g)qx}\mathcal{V}\left(\alpha_i\right)\\   
        \bra{0}\overline{q}(x)\sigma_{\alpha\beta}g_s G_{\mu\nu}(vx)q(0)\ket{0}_F &= e_q\qbarq\Bigg\{\Bigg[\left(\varepsilon_\mu - q_\mu\dfrac{\varepsilon x}{qx}\right)\left(g_{\alpha\nu}-\dfrac{1}{qx}(q_\alpha x_\nu + q_\nu x_\alpha)\right)q_\beta\\
        -&\left(\varepsilon_\mu - q_\mu\dfrac{\varepsilon x}{qx}\right)\left(g_{\beta\nu}-\dfrac{1}{qx}(q_\beta x_\nu + q_\nu x_\beta)\right)q_\alpha\\
        -&\left(\varepsilon_\nu - q_\nu\dfrac{\varepsilon x}{qx}\right)\left(g_{\alpha\mu}-\dfrac{1}{qx}(q_\alpha x_\mu + q_\mu x_\alpha)\right)q_\beta\\
        +&\left(\varepsilon_\mu - q_\mu\dfrac{\varepsilon x}{qx}\right)\left(g_{\beta\mu}-\dfrac{1}{qx}(q_\beta x_\mu + q_\mu x_\beta)\right)q_\alpha\Bigg]\\
        &\int \mathcal{D}\alpha_ie^{i(\alpha_{\Bar{q}}+v\alpha_g)qx}\mathcal{T}_1\left(\alpha_i\right)\\
        &+\Bigg[\left(\varepsilon_\alpha - q_\alpha\dfrac{\varepsilon x}{qx}\right)\left(g_{\mu\beta}-\dfrac{1}{qx}(q_\mu x_\beta + q_\beta x_\mu)\right)q_\nu\\
        -&\left(\varepsilon_\alpha - q_\alpha\dfrac{\varepsilon x}{qx}\right)\left(g_{\nu\beta}-\dfrac{1}{qx}(q_\nu x_\beta + q_\beta x_\nu)\right)q_\mu\\
        -&\left(\varepsilon_\beta - q_\beta\dfrac{\varepsilon x}{qx}\right)\left(g_{\mu\alpha}-\dfrac{1}{qx}(q_\mu x_\alpha + q_\alpha x_\mu)\right)q_\nu\\
        +&\left(\varepsilon_\beta - q_\beta\dfrac{\varepsilon x}{qx}\right)\left(g_{\nu\alpha}-\dfrac{1}{qx}(q_\nu x_\alpha + q_\alpha x_\nu)\right)q_\mu\Bigg]\\
        &\int \mathcal{D}\alpha_ie^{i(\alpha_{\Bar{q}}+v\alpha_g)qx}\mathcal{T}_2\left(\alpha_i\right)\\
        &+\dfrac{1}{qx}\left(q_\mu x_\nu - q_\nu x_\mu\right)\left(\varepsilon\alpha q_\beta - \varepsilon_\beta q_\alpha\right)\int\mathcal{D}\alpha_ie^{i(\alpha_{\Bar{q}}+v\alpha_g)qx}\mathcal{T}_3\left(\alpha_i\right)\\
        &+\dfrac{1}{qx}\left(q_\alpha x_\beta - q_\beta x_\alpha\right)\left(\varepsilon\mu q_\nu - \varepsilon_\nu q_\mu\right)\int\mathcal{D}\alpha_ie^{i(\alpha_{\Bar{q}}+v\alpha_g)qx}\mathcal{T}_4\left(\alpha_i\right)\Bigg\}\\
        \bra{0}\overline{q}(x)\sigma_{\alpha\beta} F_{\mu\nu}(vx)q(0)\ket{0}_F &=\qbarq\dfrac{1}{qx}\left(q_\alpha x_\beta - q_\beta x_\alpha\right)\left(\varepsilon_\mu q_\nu - \varepsilon_\nu q_\mu\right)\\
        &\int\mathcal{D}\alpha_ie^{i(\alpha_{\Bar{q}}+v\alpha_g)qx}\mathcal{T}^\gamma_4\left(\alpha_i\right)
    \label{photondas}
\end{align*}
where $\chi$ is the magnetic susceptibility of the quark condensate, $e_q$ is the quark charge.
