# Supplementary material for: Radiative Decays of the Spin-$\nicefrac{3}{2}$ to Spin-$\nicefrac{1}{2}$ Doubly Heavy Baryons in QCD
Source: arXiv:2306.14552 source file (2023-06-26)
Supplement: Supplementary file 2 [file appendixC.tex]

\label{chp:appndxc}
\section{Residues}
OPE part for the residues of the spin-$\nicefrac{1}{2}$ calculated as follows.

\begin{equation}
        \begin{aligned}
            \Pi^A &= \int_0^\infty ds  e^{-\frac{s}{M^2}} \int_0^1 dx \int_0^{1-x} dy\dfrac{-M^4 \delta\left(-\frac{m_Q^2}{x}-\frac{m_{Q^\prime}^2}{y}+s\right)}{128 \pi ^4}\\
            &\Big\{3 \left(5 \beta ^2+2 \beta +5\right) M^2 x y-\left(11 \beta ^2+2 \beta-13\right)m_Q m_{Q^\prime} (x+y-1)\Big\}\\
            &+\dfrac{\qbarq}{768\pi^2} \int_0^\infty ds  e^{-\frac{s}{M^2}} \int_0^1 dx \delta\left(-\frac{m_Q^2}{x}-\frac{m_{Q^\prime}^2}{\xbar}+s\right)\\
            &\Big\{\dfrac{2(1-\beta)(1+5\beta)m_0^2}{M^2}\left[\dfrac{m_Q^3\xbar}{x}+m_Q^2m_{Q^\prime}\right]\\
            &+(\beta-1)(1+5\beta)\left[8M^2m_Q\xbar+m_0^2\dfrac{m_Q}{x}\xbar(1-4x)\right]\\
            &+(\beta-1)(5+\beta)m_0^2\dfrac{m_Q}{x}+\left\{m_Q \rightarrow m_{Q^\prime}, x \rightarrow \xbar\right\}\Big\}
        \end{aligned}
    \end{equation}

    \begin{equation}
        \begin{aligned}
            \Pi^S &= \dfrac{-1}{{128 \pi ^4}}\int_0^\infty ds e^{-\frac{s}{M^2}} \int_0^1 dx \int_0^{1-x} \delta\left(-\frac{m_Q^2}{x}-\frac{m_{Q^\prime}^2}{y}+s\right) \\
            &\Big\{3 M^4 \left(\left(5 \beta ^2+2 \beta +5\right) M^2 x y-(\beta-1)^2 m_Q m_{Q^\prime} (x+y-1)\right)\Big\} \\
            &+\dfrac{\qbarq }{256 \pi^2} \int_0^\infty ds e^{-\frac{s}{M^2}} \int_0^1 dx \delta\left(-\frac{m_Q^2}{x}+\frac{m_{Q^\prime}^2}{x-1}+s\right)\left(1-\beta^2\right)\\
            &\Big\{\dfrac{6m_0^2}{M^2}\left[\dfrac{m_Q^3\xbar}{x}+m_Q^2m_{Q^\prime}\right]\\
            &+\dfrac{m_Q}{x}\left[-24M^2x\xbar+m_0^2\left(1+5x-12x^2\right)\right]+\left\{m_Q \rightarrow m_{Q^\prime}, x \rightarrow \xbar\right\}\Big\}
        \end{aligned}
    \end{equation}

    The formula for the residues was given by:

    \begin{equation}
        \lambda_{\nicefrac{1}{2}}^2 = e^{\frac{m_B^2}{M^2}} \Pi^{S(A)} 
    \end{equation}

    where the superscript $S(A)$ stands for symmetric(antisymmetric) baryon.
